# Supplementary material for: Background-aware Moment Detection for Video Moment Retrieval
Source: arXiv:2306.02728 source file (2024-09-28)
Supplement: Supplementary file 1 [file suppl.tex]

\clearpage
\setcounter{page}{1}
% \maketitlesupplementary
\appendix
\section*{Overview}

This supplementary file provides additional results not included in this paper and describes the following sections.

\begin{enumerate}
    \item Details of our experimental setup (Section \ref{sup:experimental setup})
    \item Details of our model components (Section \ref{sup:model components})
    \item Additional visualization results (Section \ref{sup:additional visualization results})
\end{enumerate}

\section{Experimental Setup}
\label{sup:experimental setup}
\subsection{Model configurations.}
We illustrate the transformer-based architecture of BM-DETR in Figure~\ref{fig:sup_model_arch}.
The encoder and decoder in our model are stacked with 3 layers of transformer block.
We set the hidden dimension of transformers as 256, and the model weights are initialized with Xavier init.
We use a fixed number of 10 learnable spans, the same number of predicted moments.
We utilize AdamW to optimize our model.
For our sampling strategy, we set the IoU threshold as 0.7 for ActivityNet-Captions and 0.5 for the other datasets to eliminate overlapping video moments.
We then extract the representations of positive and negative queries from SentenceBERT~\cite{reimers2019sbert} and compute the similarity between them.
We set the threshold of similarity as 0.5.

\subsection{Training.}
We provide more details for training each dataset: Charades-STA~\cite{gao2017tall}, ActivityNet-Captions~\cite{krishna2017dense}, TACoS~\cite{regneri2013tacos}, and QVHighlights~\cite{lei2021detecting}.
We set the batch size to 32 and select loss hyper-parameters as $\lambda_{\rm L1} = 1, \lambda_{\rm iou} = 8$, and $\lambda_{\rm cls} = 8$ for all datasets.
We extract visual features every 1s for Charades-STA and 2s for ActivityNet, TACoS, and QVHighlights.
For Charades-STA and TACoS, we set the learning rate as 2e-4. 
We set the learning rate as 1e-4 for ActivityNet-Captions and QVHighlights. 
We train the model for 100 epochs on Charades-STA and 200 epochs on the other datasets. 

\begin{figure}[t]
  \begin{center}
    \includegraphics[width=1.0\linewidth]{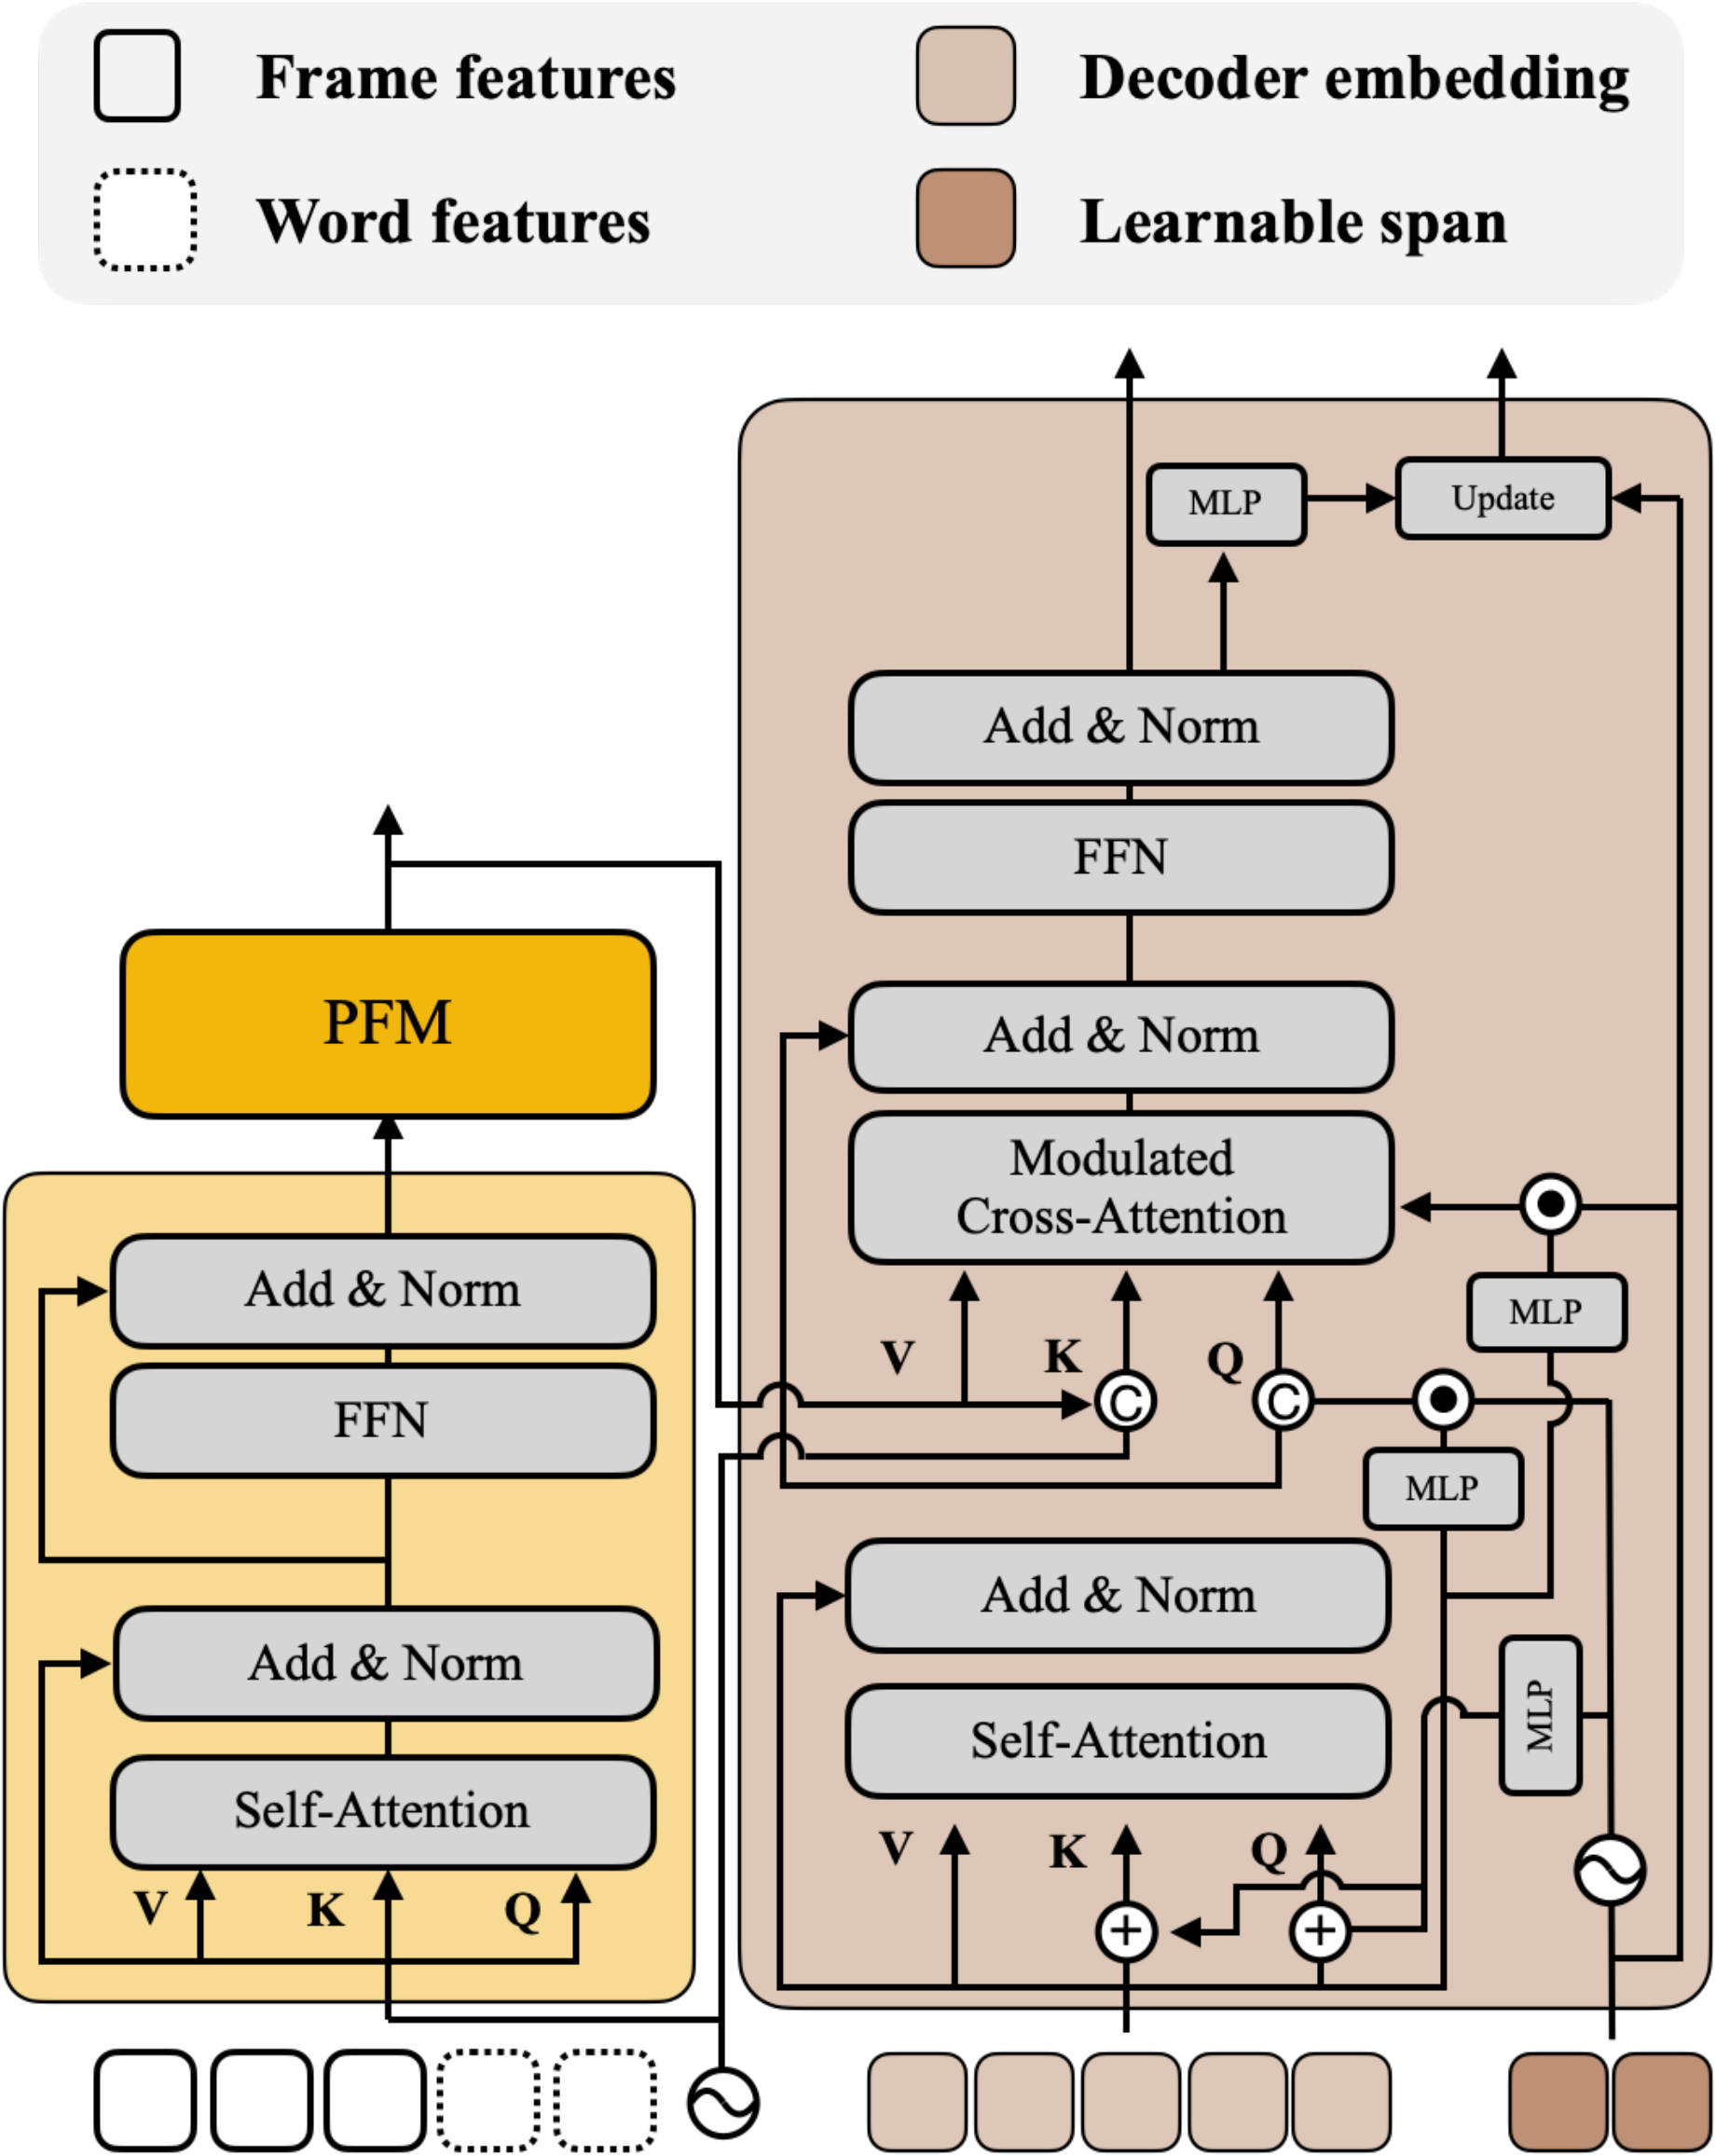}
  \end{center}
  \vspace{-3mm}
    \caption{The detailed architecture of BM-DETR.
  }
  % \vspace{-3ex}
  \label{fig:sup_model_arch}
\end{figure}

\section{Details of Model Components}
\label{sup:model components}
% In this section, we provide more details for our model components.
% \subsection{Details of our decoder.}
% Given a learnable span $S_m$, we utilize positional encoding and MLP layers to generate positional query $P_m$ as:
% \begin{equation}
%     P_m = \text{MLP}(\textit{PE}(S_m)) = \text{MLP}(\textit{PE}(c_m) \mathbin\Vert \textit{PE}(w_m)),
% \end{equation}
% where \textit{PE} means fixed positional encoding to generate sinusoidal embeddings from the learnable span.
% Two key modules in our decoder are self-attention and cross-attention.
% In the self-attention module, the queries and keys additionally take $P_m$ as:
% \begin{equation}
% Q_m = D_m + P_m, \ \ K_m = D_m + P_m, \ \ V_m = D_m,
% \end{equation}
% where $D_m$ is the decoder embedding, an input of the decoder layer.
% Each component in the cross-attention module can be represented as:
% \begin{equation}
% Q_m = (D_m \mathbin\Vert \textit{PE}(S_m) \otimes \sigma(\text{MLP}(D_m))),
% \end{equation}
% \begin{equation}
% K_m = (X_{+}' \mathbin\Vert \textit{PE}(X_{+}')), 
% \end{equation}
% \begin{equation}
%     V_m = X_{+}'.
% \end{equation}

% The learnable spans are updated layer-by-layer, and we provide the reference spans $S_{m, \rm ref}$ to utilize modulated attention, which helps to extract multimodal features with various lengths.
% \begin{equation}
%     S_{m, \rm ref} = \sigma(\text{MLP}(D_m))
% \end{equation}
% Please refer to~\cite{liu2022dab} for implementation details.

\begin{figure}[t]
  \begin{center}
    \includegraphics[width=1.0\linewidth]{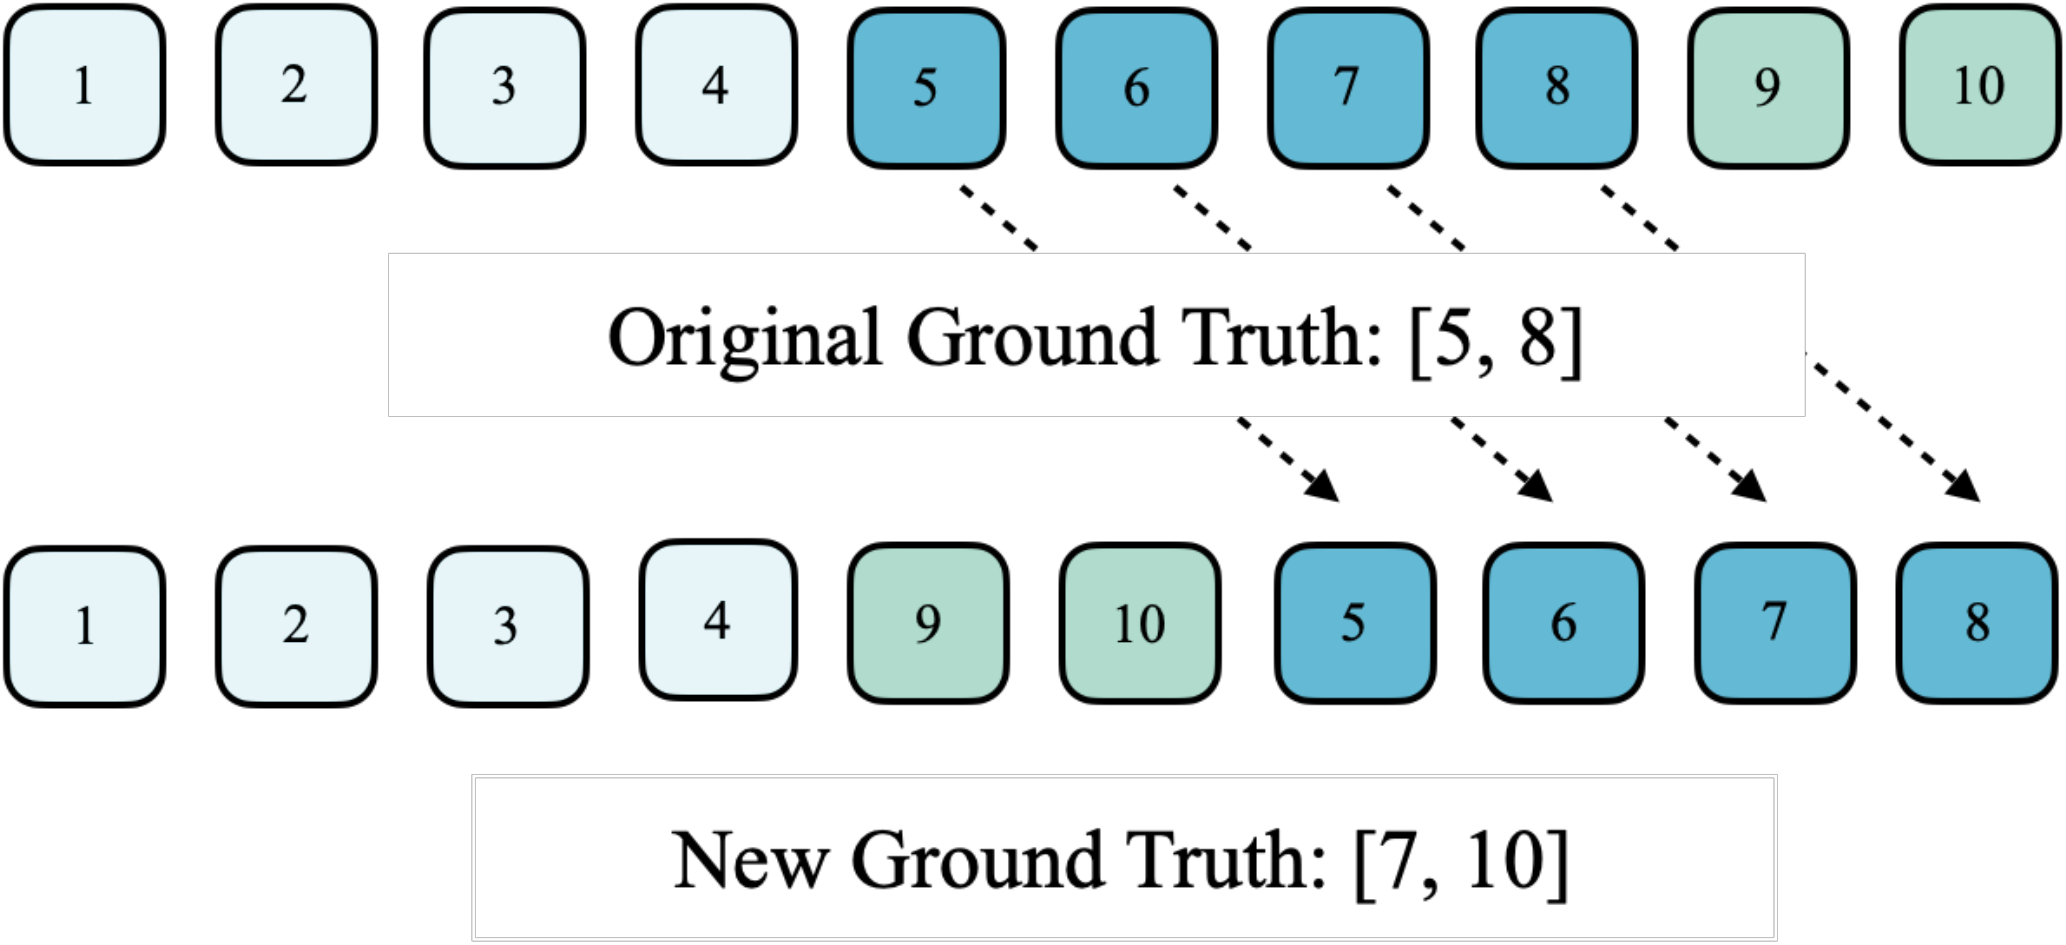}
  \end{center}
  \vspace{-3mm}
    \caption{Visualization of temporal shifting method. When temporal shifting is applied to the video, we randomly move the frames in the ground-truth moment while keeping the sequence of frames
  }
  % \vspace{-3ex}
  \label{fig:sup_ts}
\end{figure}

\begin{figure}[t]
  \begin{center}
    \includegraphics[width=1.0\linewidth]{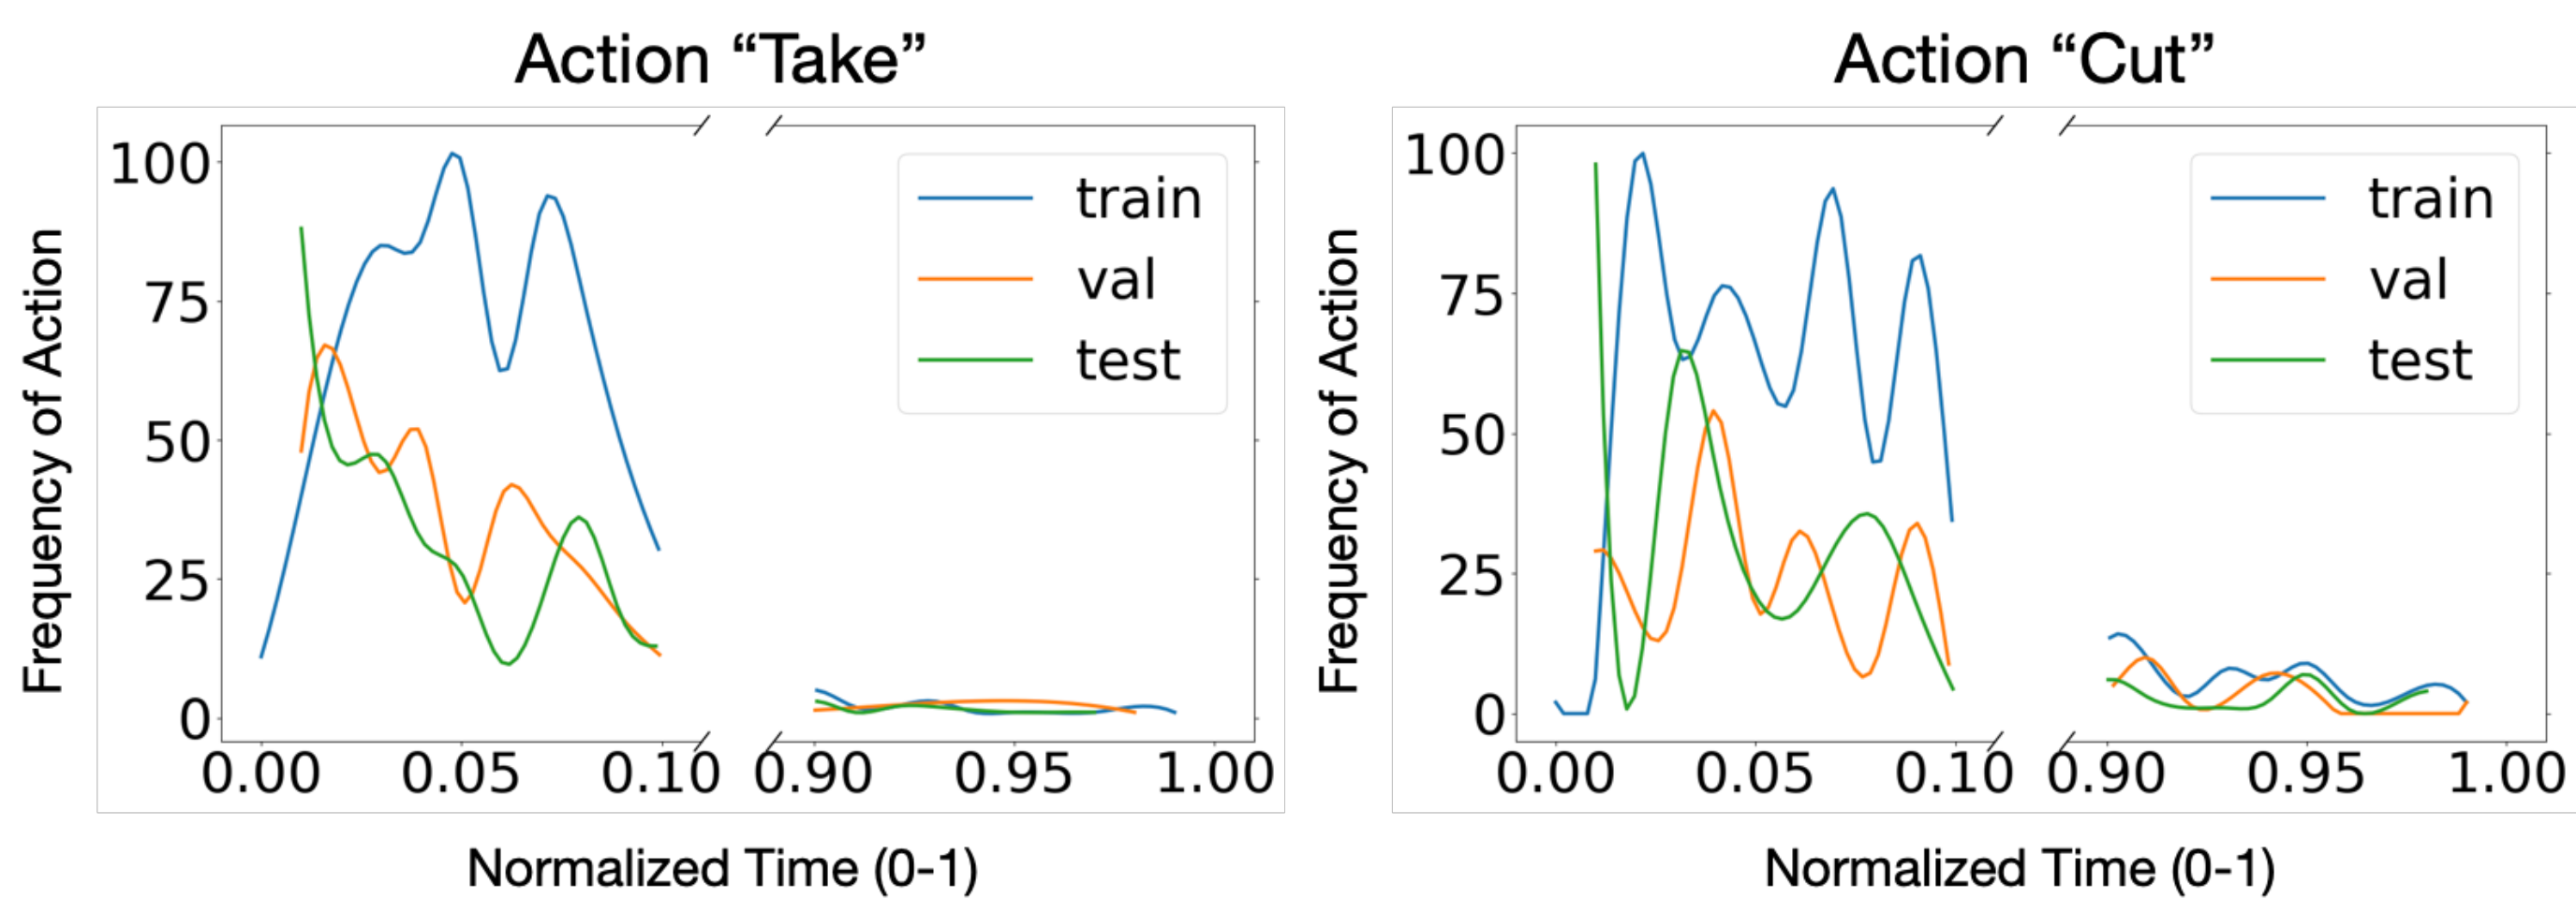}
  \end{center}
  \vspace{-3mm}
    \caption{Normalized temporal distribution of action in TACoS.
  }
  % \vspace{-3ex}
  \label{fig:sup_experiment_ts}
\end{figure}

\subsection{Details of temporal shifting.}
Let us suppose the target video $V$ has $L$ frames as $V=\{f_i\}_{i=1}^{L}$, and the length of the ground-truth moment is $l$ ($l < L$).
First, we randomly select a new start/end index $s_{start}$/$s_{end}$ as follows: 
\begin{flalign}
    s_{start} &\sim {U}(0, L - l), ~~ l \in \mathcal{Z}\\
    s_{end} &= s_{start} + l.
\end{flalign}
Then we shift frames in the ground-truth moment to the new ground-truth moment while maintaining the sequence of frames.
For ease of explanation, in Figure~\ref{fig:sup_ts}, let us define the given video $V$ contains 10 frames with 1 FPS, and the start and end times of the ground-truth moment in $V$ are 5s and 8s.
Then we randomly select $s_{start}$ and $s_{end}$ as 7s and 10s.
Finally, the ground-truth moment (5s, 8s) is changed to the new ground-truth moment (7s, 10s).

As discussed before, we further investigate the temporal shifting's inconsistent impact.
We find that TACoS videos have 60 times more queries on average than Charades-STA (135.2 vs 2.3), and due to the nature of cooking videos, learning procedural information from these queries appears to be crucial.
As depicted in Figure~\ref{fig:sup_experiment_ts}, specific actions consistently appear in the early video segments but diminish in the later parts.
Consequently, temporal shifting may not yield benefits for learning these temporal relationships.
We will develop effective temporal augmentation methods for VMR in our future work.
\begin{figure}[t]
  \begin{center}
    \includegraphics[width=0.8\linewidth]{figs_sup/Additional Visualizations.pdf}
  \end{center}
  \vspace{-3mm}
    \caption{
   Four visualization examples of our model’s moment prediction. 
   We show predicted and ground-truth moments and present the attention scores $\bf o$ below.
  }
  \label{fig:additional visualizations}
    % \vspace{-3ex}
\end{figure}

\section{Additional Visualization Results}
\label{sup:additional visualization results}
We provide further insight into how our model addresses the weak alignment problem in the video, providing additional support for the results in Table~\ref{tbl:prob}. 
Figure~\ref{fig:visual example of prob} presents the predictions of each model for a given video.
The query describes only one person despite two individuals in the video, and the terms ``person'' and ``window'' in the query are present not only in the target moment but throughout the entire video.
Our baseline model fails to predict the target moment due to the lack of clear distinction in frame probabilities between the ground-truth moment. 
In contrast, BM-DETR provides accurate predictions by assigning higher probabilities to frames in the ground-truth moments than to other frames, mitigating the weak alignment problem effectively.
Additionally, we provide four additional visualization results of our model’s prediction on QVHighlights in Figure~\ref{fig:additional visualizations}.
% In Figure~\ref{fig:visualization of charades_anet}, we visualize our model's predictions on videos in Charades-STA and ActivityNet-Captions. 
% In Charades-STA, queries typically focus on interactions between people and objects, particularly ``laptops,'' observed throughout the video. 
% Our model effectively identifies and accurately predicts temporal moments for each event. 
% For ActivityNet-Captions, queries share similar concepts, all describing the action ``dancing.''
% In this case, we found that our model does not treat these similar queries as negatives, even though their temporal locations differ, resulting in inaccurate predictions. 
% This kind of issue degrades the effectiveness of our approach, and our future work will address it.

\begin{figure}[t]
  \begin{center}
    \includegraphics[width=0.9\linewidth]{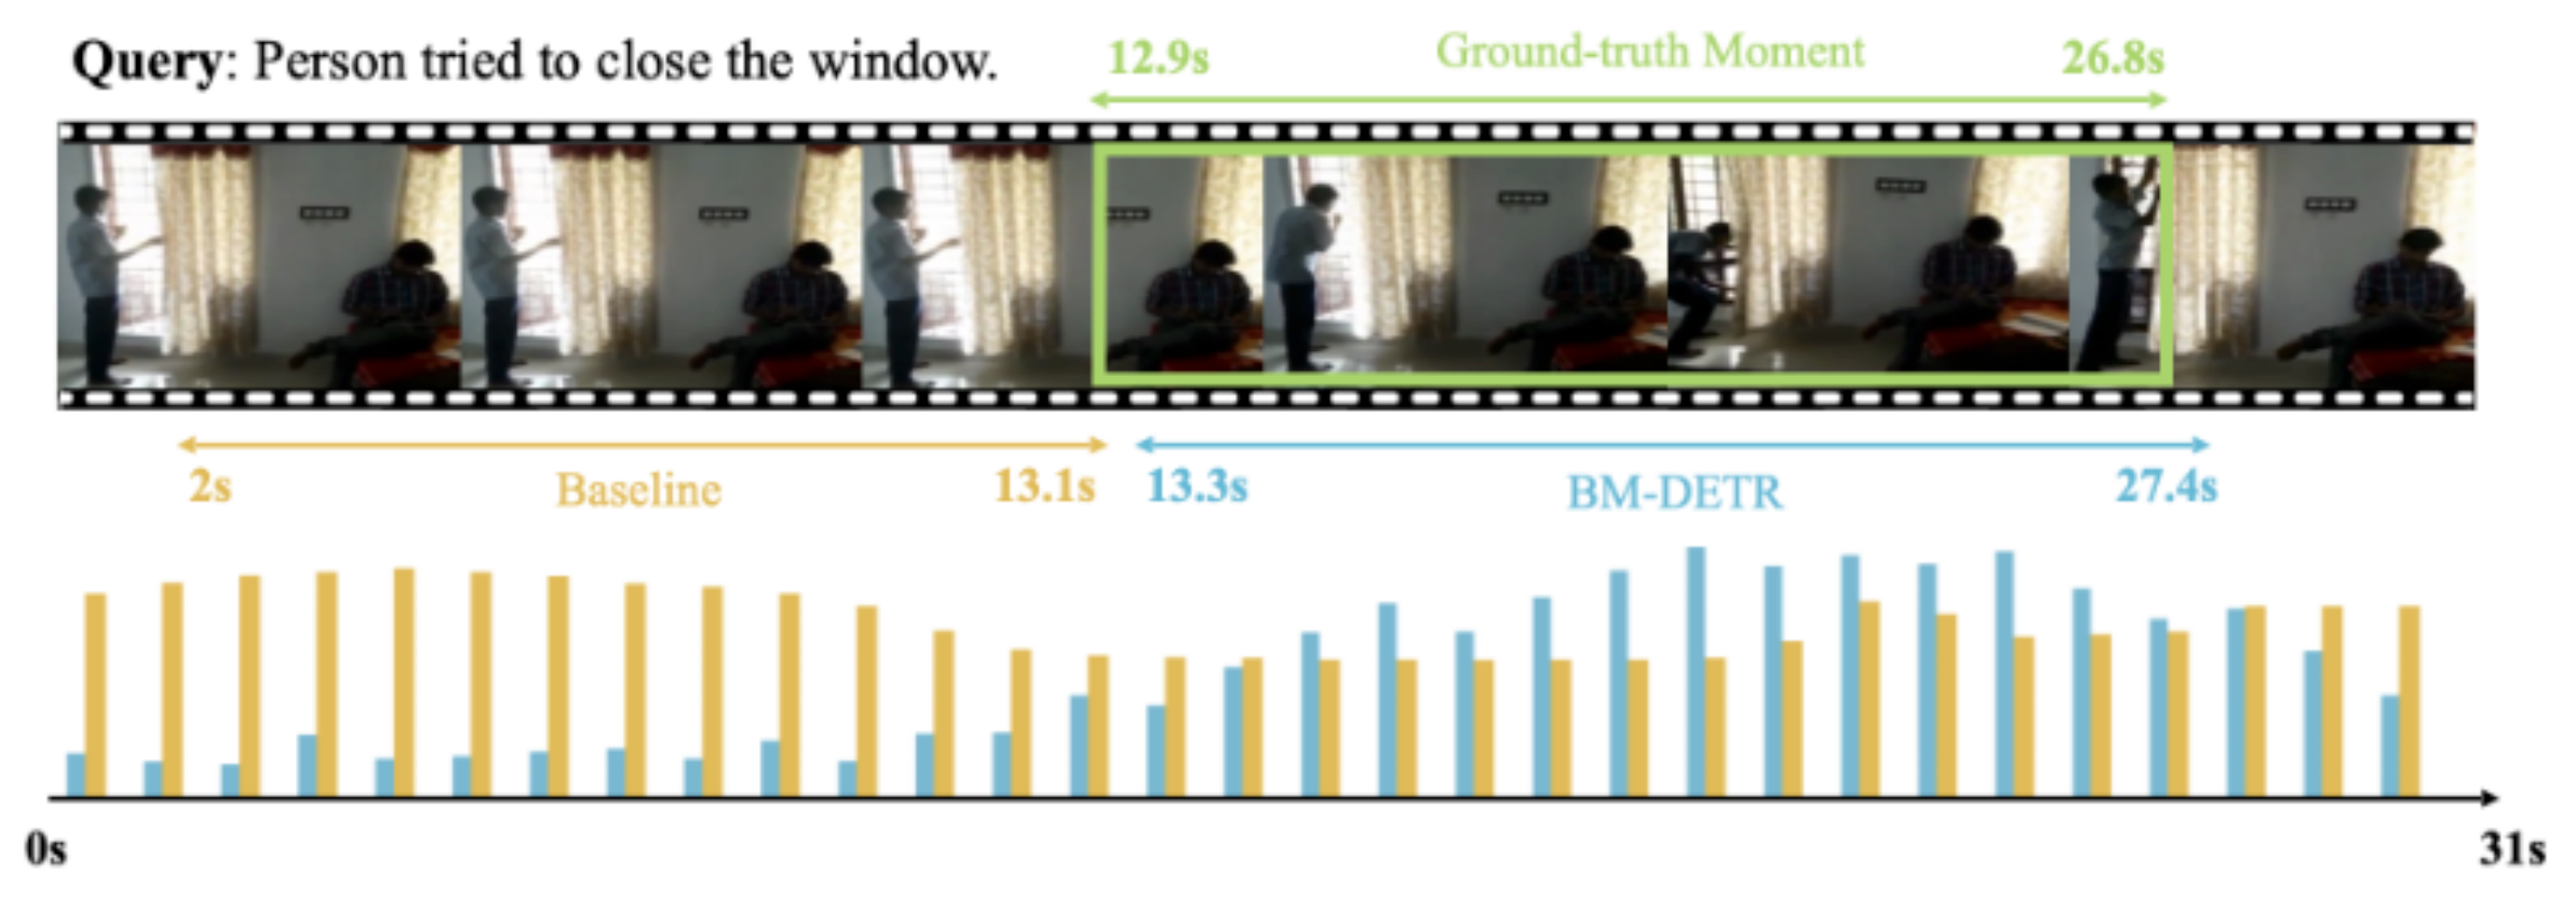}
  \end{center}
  \vspace{-4mm}
    \caption{
  Visualization of model's predictions.
  We present the frame probability $\bf{p}$ below the ground-truth and predicted moments.
  }
  \label{fig:visual example of prob}
\end{figure}
